# Supplementary material for: Generation and controllable switching of superradiant and subradiant states in a 10-qubit superconducting circuit
Source: arXiv:1907.13468 source file (2019-07-30)
Supplement: Supplementary file 1 [file SI.pdf]

# Supplementary material for "Generation and controllable switching between superradiant and subradiant states in a 10-qubit superconducting circuit"

Zhen Wang[1], Hekang Li[2], Wei Feng[1], Xiaohui Song[2], Chao Song[1], Wuxin Liu[1], Qiujiang Guo[1], Xu Zhang[1], Hang Dong[1], Dongning Zheng[2,3],* H. Wang[1],† and Da-Wei Wang[1,3]‡

[1]*Interdisciplinary Center for Quantum Information, State Key Laboratory of Modern Optical Instrumentation, and Zhejiang Province Key Laboratory of Quantum Technology and Device, Department of Physics, Zhejiang University, Hangzhou 310027, China,*

[2] *Institute of Physics, Chinese Academy of Sciences, Beijing 100190, China,*

[3] *CAS Center for Excellence in Topological Quantum Computation, University of Chinese Academy of Sciences, Beijing 100190, China*

(Dated: July 24, 2019)

* dzheng@iphy.ac.cn

† hhwang@zju.edu.cn

‡ dwwang@zju.edu.cn

## NOTE 1: SUPERRADIANT AND SUBRADIANT STATES OF MANY QUBITS COUPLED TO A RESONATOR

The interaction Hamiltonian of many qubits coupled to the same resonator is,

$$H_I/\hbar = g(S^+a + a^\dagger S^-), \tag{1}$$

where $S^{+(-)} = \sum_{j=1}^{N} \sigma_j^{+(-)}$ is the collective spin raising (lowering) operator. The first excited state is generated by applying the interaction Hamiltonian to the ground state $|G_N\rangle = |0_1 0_2 ... 0_N\rangle$,

$$|B_N\rangle = \frac{1}{\sqrt{N}} \sum_{j=1}^{N} |0_1 0_2 ... 1_j ... 0_N\rangle, \tag{2}$$

which is the single-photon superradiant state. The coupling strength between $|B_N\rangle$ and $|G_N\rangle$ is $\langle B_N|H_I|G_N\rangle = \sqrt{N}ga$, i.e., enhanced by $\sqrt{N}$ times compared to the case of single qubit. We can apply the raising operator to $|B_N\rangle$ to generate higher excited states in the superradiant subspace. The states in this subspace can be described by a spin-$N/2$ system [1].

The single-photon subradiant states are decoupled from the ground state. To write them down are there many ways [2–4], among which the proposal in ref. [4] can be directly used in switching between superradiant and subradiant states. The key is to keep the probability amplitudes of the component states in $|B_N\rangle$ unchanged while locally modulate the phase of each component state. The subradiant states are

$$|D_N^n\rangle = \frac{1}{\sqrt{N}} \sum_{j=1}^{N} e^{-2ijn\pi/N} |0_1 0_2 ... 1_j ..., 0_N\rangle \tag{3}$$

where $n = 1, 2, ..., N-1$. There are $N-1$ single-photon subradiant states in total. We investigate $|D_N^1\rangle \equiv |D_N\rangle$ in the main text and all other subradiant states can be similarly generated and tested. $|D_N^n\rangle$ are the ground states in subradiant subspaces. Other states in these subspaces are obtained by applying $S^+$ to $|D_N^n\rangle$. These states obey the symmetry of a spin-$(N/2-1)$ particle. In the following, we show more details of the superradiant and subradiant subspaces of 4 qubits.

For $N = 4$, applying $S^+$ to the ground state $|G_4\rangle = |0000\rangle$ yields (we ignore the subscript $n$ labeling the $n$th spin for simplicity)

$$|B_4\rangle = \frac{1}{2}[|1000\rangle + |0100\rangle + |0010\rangle + |0001\rangle], \tag{4}$$

which is the 4-qubit single-photon superradiant state. The three single-photon subradiant states are

$$|D_4^1\rangle = \frac{1}{2}[|1000\rangle + e^{-i\pi/2}|0100\rangle + e^{-i\pi}|0010\rangle + e^{-i3\pi/2}|0001\rangle], \tag{5}$$

$$|D_4^2\rangle = \frac{1}{2}[|1000\rangle + e^{-i\pi}|0100\rangle + e^{-i2\pi}|0010\rangle + e^{-i3\pi}|0001\rangle], \tag{6}$$

and

$$|D_4^3\rangle = \frac{1}{2}[|1000\rangle + e^{-i3\pi/2}|0100\rangle + e^{-i3\pi}|0010\rangle + e^{-i9\pi/2}|0001\rangle]. \tag{7}$$

It is easy to verify that $S^-|D_4^n\rangle = 0$ $(n = 1, 2, 3)$, which means these states cannot emit photons. However, they can still be excited to other states, e.g., $S^+|D_4^1\rangle = \sqrt{2}|E_4^1\rangle$, where

$$|E_4^1\rangle = \frac{1}{2}[e^{-i\pi/4}|1100\rangle + e^{i\pi/4}|1001\rangle - e^{i\pi/4}|0110\rangle - e^{-i\pi/4}|0001\rangle]. \tag{8}$$

The coupling strength between $|D_4^1\rangle$ and $|E_4^1\rangle$ is $\sqrt{2}g$, the same as the one between $|B_2\rangle$ and $|G_2\rangle$, which is verified by comparing the Rabi frequencies in Fig. 3 (b) and Fig. 4 (b). $|D_4^n\rangle$ and $|E_4^n\rangle$ are the ground and first excited states

TABLE S1. Parameters of the 10-qubit superconducting circuit. Sweet point is the flux-insensitive point where the resonant frequency of the qubit reaches maximum. Idle point is where the qubit is initialized and measured. $T_1$ is the energy relaxation time and $T_2$ is the dephasing time for a stand-alone qubit. $g_i$ is the coupling strength between $Q_i$ and $R$.

| | $Q_0$ | $Q_1$ | $Q_2$ | $Q_3$ | $Q_4$ | $Q_5$ | $Q_6$ | $Q_7$ | $Q_8$ | $Q_9$ |
|---|---|---|---|---|---|---|---|---|---|---|
| Sweet point (GHz) | 6.21 | 6.29 | 6.20 | 6.15 | 6.15 | 6.45 | 6.33 | 6.56 | 6.60 | 6.49 |
| Idle point (GHz) | 5.225 | 5.159 | 5.479 | 5.507 | 5.515 | 5.542 | 5.437 | 5.418 | 5.168 | 5.485 |
| $g_i/2\pi$ (MHz) | 13.3 | 13.8 | 12.8 | 14.0 | 13.4 | 13.4 | 13.8 | 12.7 | 14.0 | 13.4 |
| $T_1$ ($\mu$s) | 13.1 | 17.9 | 16.5 | 24.9 | 26.4 | 15.4 | 42.1 | 35.8 | 92.2 | 43.2 |
| $T_2$ ($\mu$s) | 0.7 | 1.1 | 1.0 | 0.8 | 1.1 | 1.0 | 1.2 | 1.0 | 1.3 | 1.0 |

of three spin-1 subradiant subspaces, which include 9 states. Apart from these states and the 5 states in the spin-2 superradiant subspace, there are 2 singlet states left for all possible 16 states of 4 qubits. They are

$$|S_4\rangle = \frac{1}{2}[|1100\rangle + e^{i\pi}|0110\rangle + e^{i2\pi}|0011\rangle + e^{i3\pi}|1001\rangle], \tag{9}$$

and

$$|R_4\rangle = \frac{1}{\sqrt{6}}[\frac{1}{\sqrt{2}}(|1100\rangle + |0110\rangle + |0011\rangle + |1001\rangle) - \sqrt{2}(|1010 + |0101\rangle\rangle)]. \tag{10}$$

These two states satisfy $S^+|S(R)_4\rangle = 0$ and $S^-|S(R)_4\rangle = 0$, which means that they can neither emit nor absorb photons. We verify the properties of $|S_4\rangle$ in Fig. 4.

## NOTE 2: DEVICE CHARACTERISTICS

The detailed experimental setup such as XY control, Z control and qubit readout can be found in Ref. [5]. Device parameters are summarized in Table S1. The resonant frequency $\omega_R/2\pi$ of the central bus resonator $R$ is fixed at around 5.69 GHz. In the experiment, the qubit idle frequencies are more than 140 MHz below $\omega_R/2\pi$.

### Qubit-resonator coupling strength

We obtain the qubit-resonator coupling strength by measuring the vacuum Rabi oscillation as a function of the Z pulse amplitude (ZPA). We excite the qubit, e.g., $Q_i$, to $|1\rangle$ and then apply the rectangular Z pulse for 1000 ns, with the pulse height noted as ZPA which effectively tunes the qubit frequency, to measure the swapping dynamics between $Q_i$ and $R$. We estimate the coupling strength $g_i$ and the on-resonance ZPA value from fitting the oscillation patterns. During the measurement, all the other qubits are detuned far from $R$ in frequency and their effects can be neglected.

### Relaxation time ($\mathbf{T_1}$) and dephasing time ($\mathbf{T_2}$)

In Fig. S1(a), we plot the excited state ($|1\rangle$) population $P_1$ of each qubit as a function of delay. By fitting the damping curvatures according to $P_1(t) \propto e^{-t/T_1}$, we obtain the energy relaxation time ($T_1$) of each qubit. Figure S1(b) shows the Ramsey fringe measurement of all qubits. We fit the damping Ramsey envelope according to $P_1^E(t) \propto 0.5 + 0.5e^{-t/2T_1-(t/T_2)^2}$ to obtain the dephasing time ($T_2$), where $T_1$ is from the previous fitting. Here the dephasing time is measured for each individual qubit. However, in our experiment all the qubits are on resonance with $R$ to form a coupled system, whose eigenenergies depend weakly on each qubit flux[6]. As a result, the effective dephasing time should be longer.

### Qubit-qubit crosstalk coupling strength

To minimize the qubit-qubit crosstalk coupling $g_{ij}$, we implement a design with the qubits being separated as far as possible while they surround the central bus resonator, as shown in Fig. 1(a) of the main text. To estimate $g_{ij}$ between

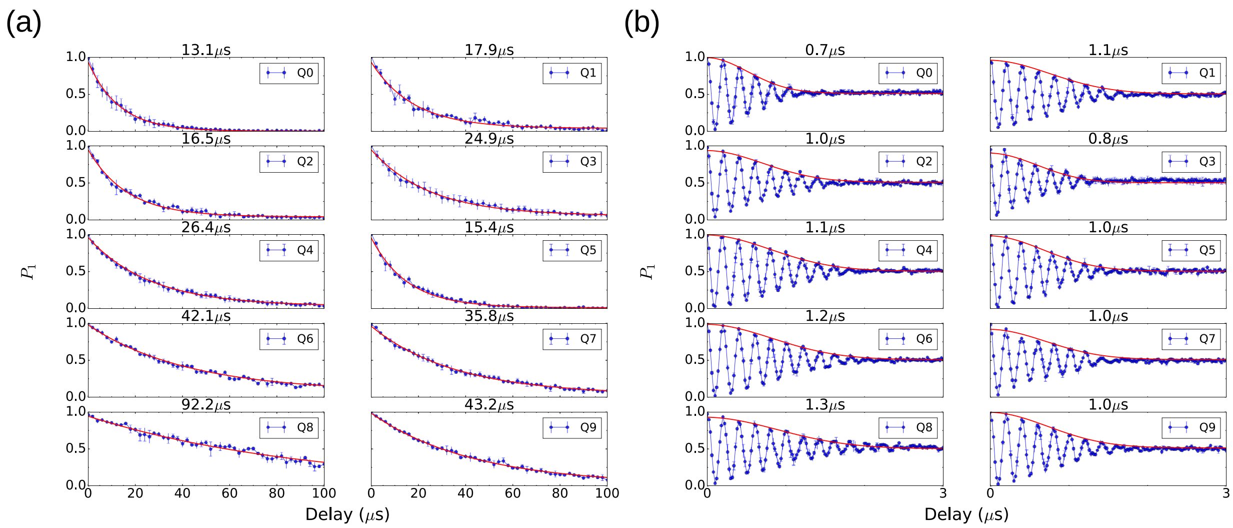


FIG. S1. (a) Relaxation time ($T_1$) and (b) dephasing time ($T_2$) measurements at the idle point for each qubit. Blue dots are experimental data and red solid lines are fitting results. The estimated $T_1$ and $T_2$ values are listed on top of the corresponding plots.

$Q_i$ and $Q_j$, we bias these two qubits to about $|\Delta|$ below $\omega_{\rm R}$ while all the other qubits are at the respective sweet points, following which we record their swapping dynamics as function of both delay and their relative frequency detuning to estimate the effective qubit-qubit coupling strength. After subtracting the contribution due to the resonator's mediation, i.e., $\sim g_i g_j/\Delta$, we obtain $g_{ij}$. Most $g_{ij}$ values estimated this way are no more than 0.2 MHz, which are much less than the typical values of $g_i$ ($\sim$ 13 MHz).

## NOTE 3: EXPERIMENTAL DETAILS

### Measurement of the resonator photon population

When no more than a single photon excitation is in the resonator $R$, we can apply a rectangular Z pulse on $Q_0$, initialized in its ground state, to couple it resonantly with $R$ for a time $t_{\rm iSWAP}$, which transfers the resonator photon into $Q_0$. $P_1$ of $Q_0$ gives the photon population in $R$. When more than a single excitation are in $R$, we can use the method in Ref.[7] to measure the photon population in the resonator. We allow $Q_0$ to interact with $R$ resonantly for up to 1000 ns. By analyzing the resulting swapping dynamics, we can obtain the probability populations in different photon eigenstates, i.e., Fock states, of the resonator.

### Calibrating the phase factors in subradiance/superradiance

Taking the three-qubit case as an example, after the first rectangular Z pulses to all three qubits as shown in Fig. 1(b) of the main text, the state can be written as

$$|\psi\rangle = \frac{1}{\sqrt{3}}(|001\rangle + e^{i\varphi_2}|010\rangle + e^{i\varphi_3}|100\rangle) \otimes |0_R\rangle \, , \tag{11}$$

where $\varphi_2$ and $\varphi_3$ are the accumulated dynamical phases with respect to the first term. We can modify these phases by applying single-qubit phase gates (small Z pulses with variable amplitudes). Figure S2 displays the measured resonator photon population as a function of $\varphi_2$ and $\varphi_3$, after the resonator, initially in $|0_R\rangle$, collectively interacts with the three qubits in the state described by Eq. (11) for a duration of $\pi/2\sqrt{3}g$. For $\varphi_2 = \varphi_3 = 0$, the three qubits are in superradiance and can radiate the single photon excitation into $R$, yielding

$$|\psi_1\rangle = \frac{1}{\sqrt{3}}(|000\rangle + |000\rangle + |000\rangle) \otimes |1_R\rangle \, . \tag{12}$$

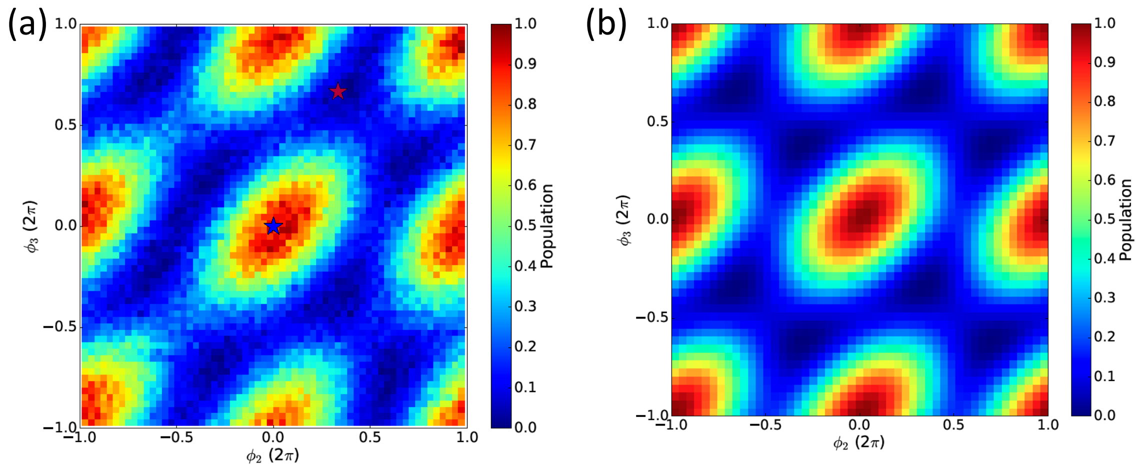


FIG. S2. (a) Experimental results of the resonator photon population as a function of $\varphi_2$ and $\varphi_3$ after the resonator, initially in vacuum, resonantly interacts with the three qubits in the state in Eq. (11) for a duration of $\pi/2\sqrt{3}g$. For superradiant state ($\varphi_2 = \varphi_3 = 0$), the photon is completely transferred to $R$ (blue star), while for subradiant state ($\varphi_2 = 2\pi/3$, $\varphi_3 = 4\pi/3$), the photon is stored in the subradiant state (red star). (b) Numerical simulation results in comparison with the data in (a).

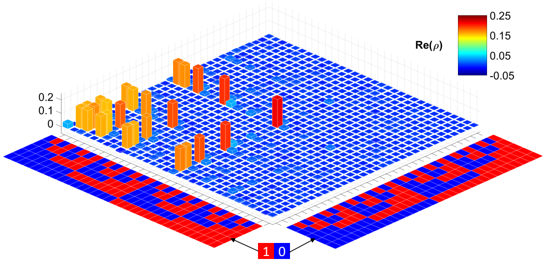


FIG. S3. Density matrix of the 5-qubit superradiant state using quantum state tomography. The state fidelity is approximately 84%.

This process is marked by a blue star in Fig. S2(a). For $\varphi_2 = 2\pi/3$, and $\varphi_3 = 4\pi/3$, the three qubits are in subradiance and no radiation occurs, so that

$$|\psi_2\rangle = \frac{1}{\sqrt{3}}(|100\rangle + e^{i2\pi/3}|010\rangle + e^{i4\pi/3}|001\rangle) \otimes |0_R\rangle\,. \tag{13}$$

In this process no photon is transferred to $R$, which is marked by a red star in Fig. S2(a). Numerical results are shown in Fig. S2(b), which are in accord with the experimental data.

Here we also display the experimental density matrix of the 5-qubit superradiant state in Fig. S3, and the pulse sequences used for the data in Fig. 4 of the main text in Figs. S4 and S5.

[1] Robert H Dicke, "Coherence in spontaneous radiation processes," Phys. Rev. **93**, 99 (1954).
[2] A. Maser, U. Schilling, T. Bastin, E. Solano, C. Thiel, and J. von Zanthier, "Generation of total angular momentum eigenstates in remote qubits," Phys. Rev. A **79**, 033833 (2009).
[3] Marlan O Scully, "Collective lamb shift in single photon dicke superradiance," Phys. Rev. Lett. **102**, 143601 (2009).
[4] Philip A Vetter, Luojia Wang, Da-Wei Wang, and Marlan O Scully, "Single photon subradiance and superradiance revisited: a group theoretic analysis of subradiant states," Physica Scripta **91**, 023007 (2016).

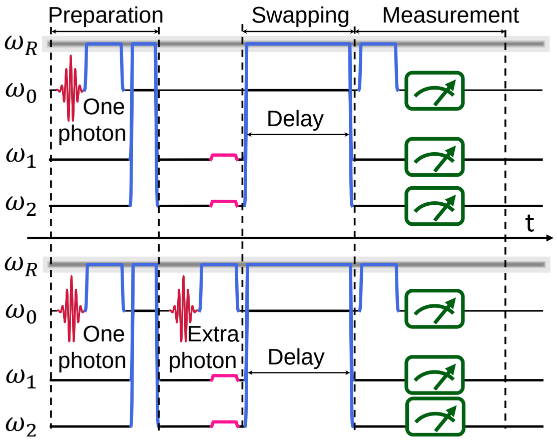


FIG. S4. Pulse sequences used to introduce one photon (top panel) and two photons (bottom panel) into the subradiant state $|D_N\rangle$ for N=2. In both sequences, we use the same process to generate the single-excitation subradiant states in the preparation stage. To introduce an extra photon into $R$, we first excite Q$_0$ again and then apply a Z pulse with a duration of $t_{\rm iSWAP} \approx \pi/2g$ to transfer the excitation into $R$. After that, we immediately apply a series of big Z pulses with different delays followed by qubit readout to observe the collective swapping dynamics. The experimental results are shown in Figs. 4(a) and (b).

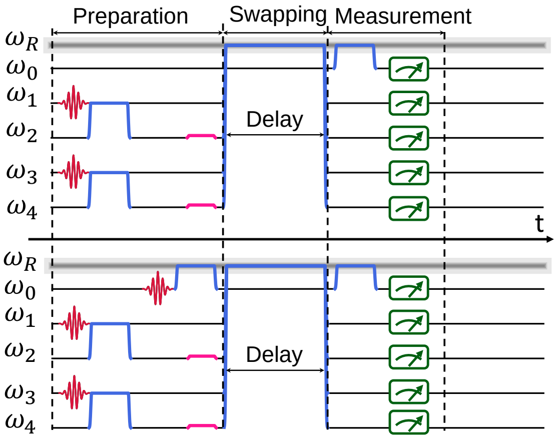


FIG. S5. Pulse sequences for generating the 4-qubit singlet subradiant state (top panel) and to introduce one extra photon into $R$ (bottom panel). The Einstein-Podolsky-Rosen (EPR) state $(|01\rangle - |10\rangle)/\sqrt{2}$ is generated by first exciting one qubit ($Q_1$ for example) and then tuning another qubit ($Q_2$) on resonance with $Q_1$ for $t_{\rm iSWAP} \approx \pi/2g_{12}$. Here $g_{12}$ is the coupling strength between $Q_1$ and $Q_2$. The two pairs of EPR states ($Q_1$-$Q_2$ and $Q_3$-$Q_4$) are generated simultaneously. The only difference between the top and bottom panels is that one extra photon is introduced into $R$ in the bottom panel using the same procedure as that described in the caption of Fig. S4. The experimental results are shown in Figs. 4(c) and (d).

[5] Chao Song, Kai Xu, Wuxin Liu, Chui-ping Yang, Shi-Biao Zheng, Hui Deng, Qiwei Xie, Keqiang Huang, Qiujiang Guo, Libo Zhang, Pengfei Zhang, Da Xu, Dongning Zheng, Xiaobo Zhu, H. Wang, Y.-A. Chen, C.-Y. Lu, Siyuan Han, and Jian-Wei Pan, "10-qubit entanglement and parallel logic operations with a superconducting circuit," Phys. Rev. Lett. **119**, 180511 (2017).

[6] Kai Xu, Jin-Jun Chen, Yu Zeng, Yu-Ran Zhang, Chao Song, Wuxin Liu, Qiujiang Guo, Pengfei Zhang, Da Xu, Hui Deng, Keqiang Huang, H. Wang, Xiaobo Zhu, Dongning Zheng, and Heng Fan, "Emulating many-body localization with a superconducting quantum processor," Phys. Rev. Lett. **120**, 050507 (2018).

[7] H. Wang, M. Hofheinz, M. Ansmann, R. C. Bialczak, E. Lucero, M. Neeley, A. D. O'Connell, D. Sank, J. Wenner, A. N. Cleland, and John M. Martinis, "Measurement of the decay of fock states in a superconducting quantum circuit," Phys. Rev. Lett. **101**, 240401 (2008).
